# Supplementary material for: Readout Guidance: Learning Control from Diffusion Features
Source: arXiv:2312.02150 source file (2024-04-02)

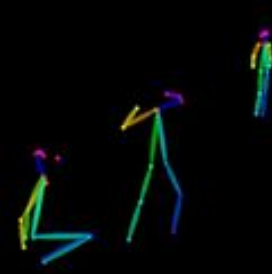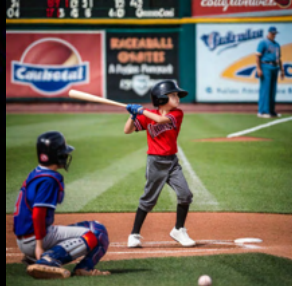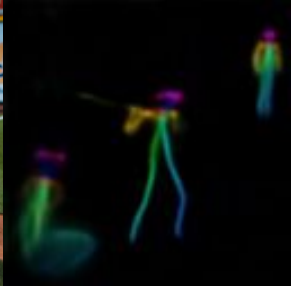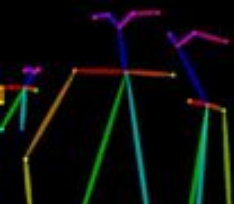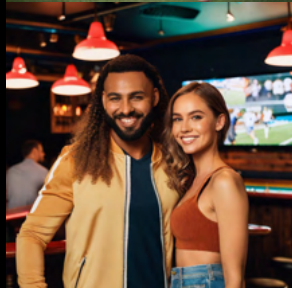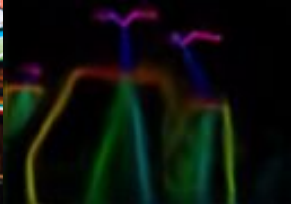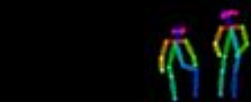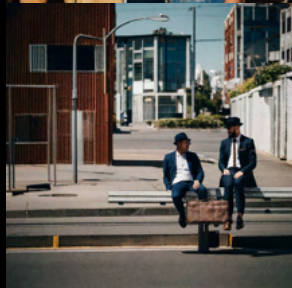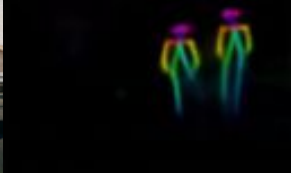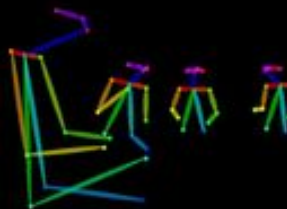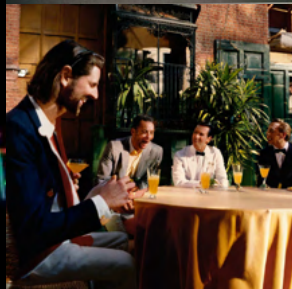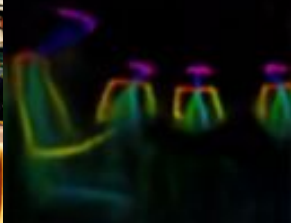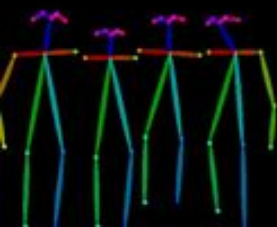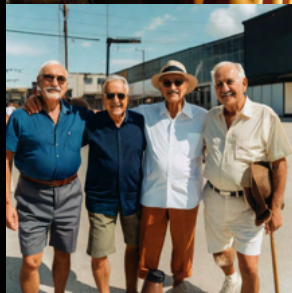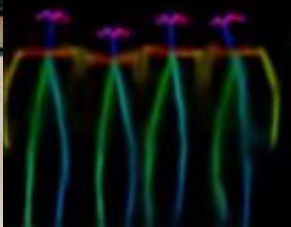

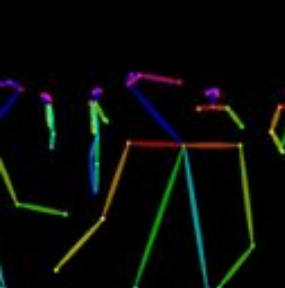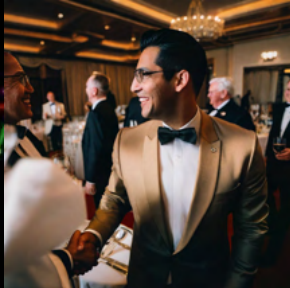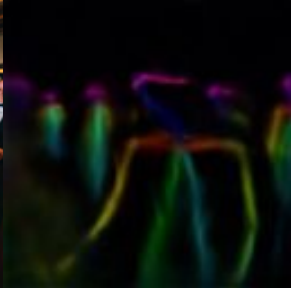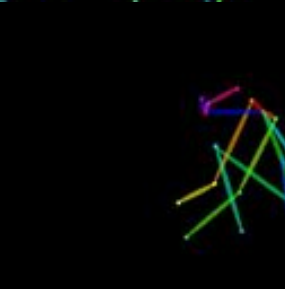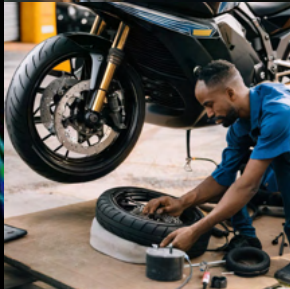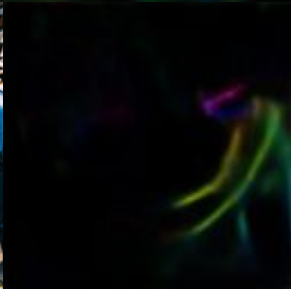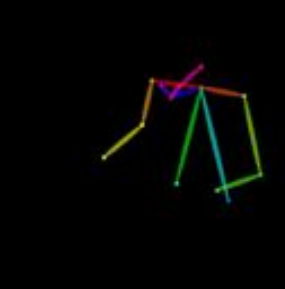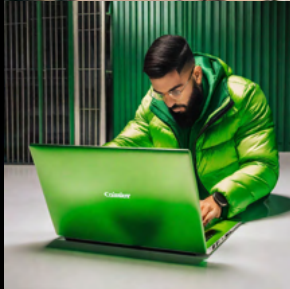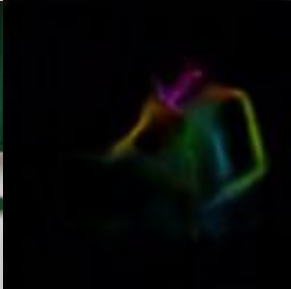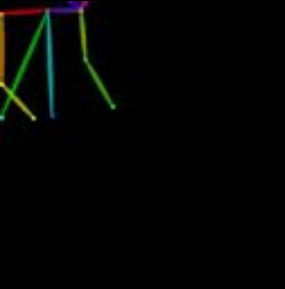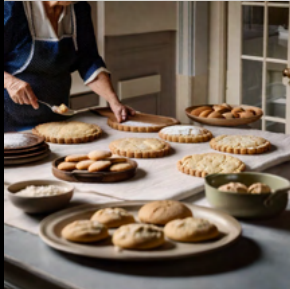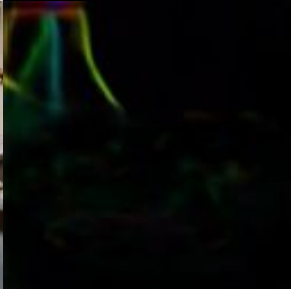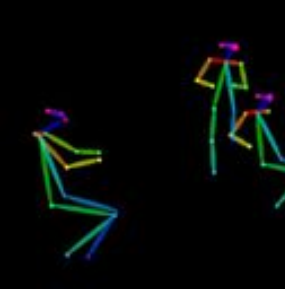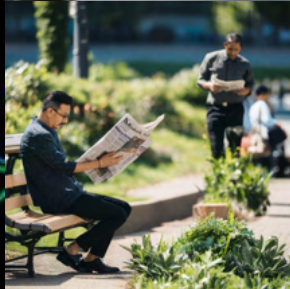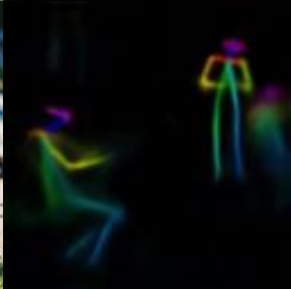

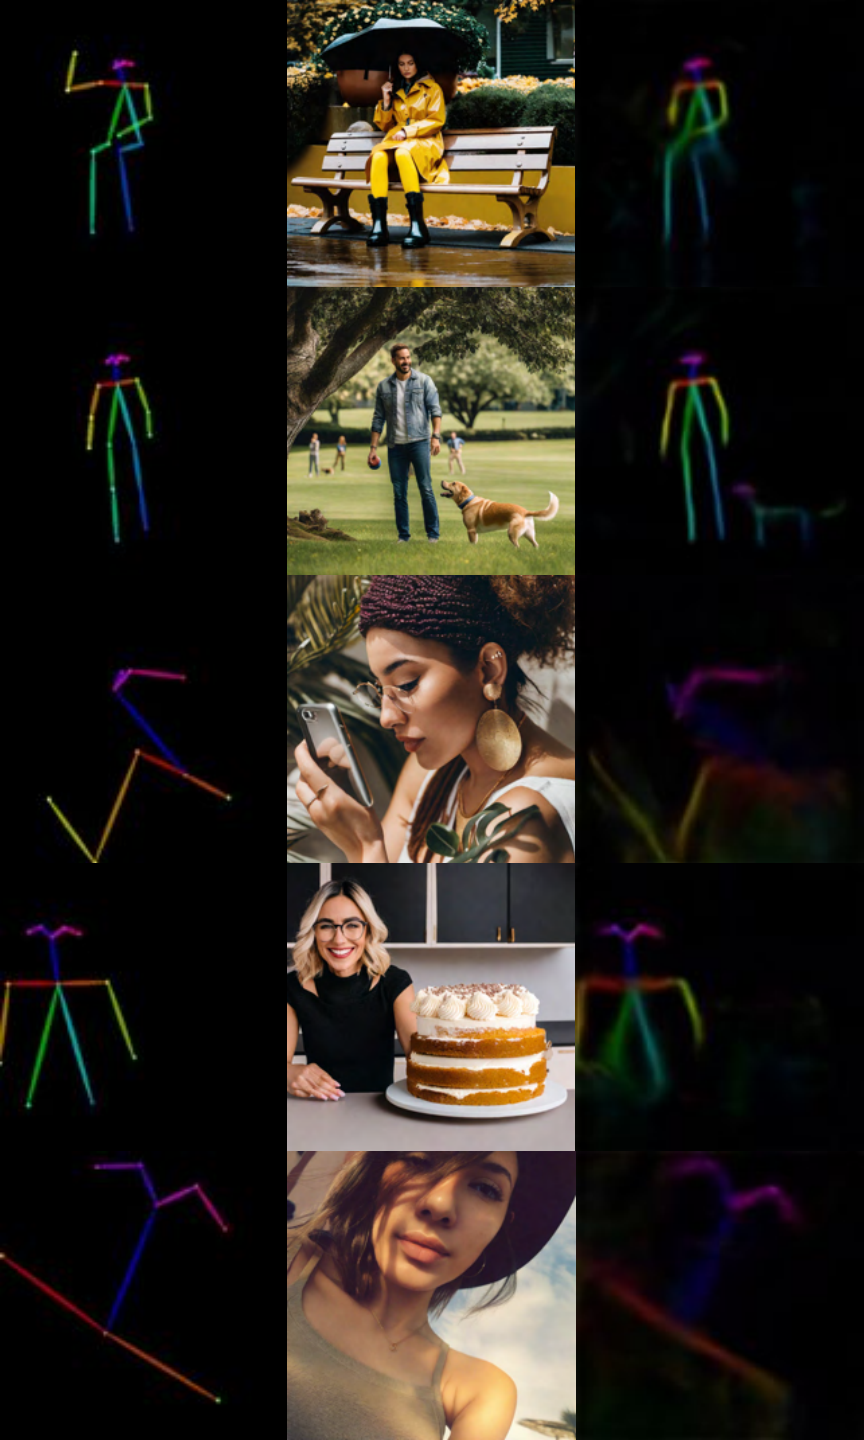

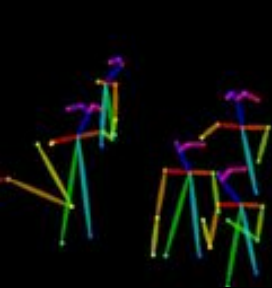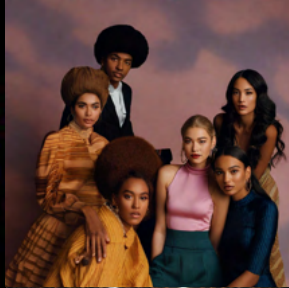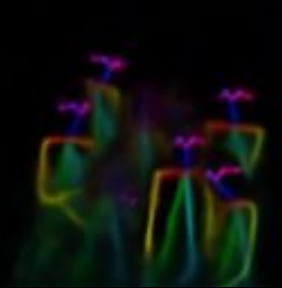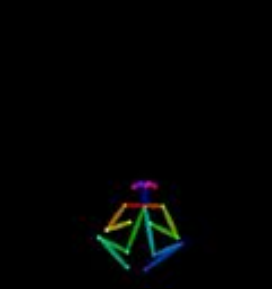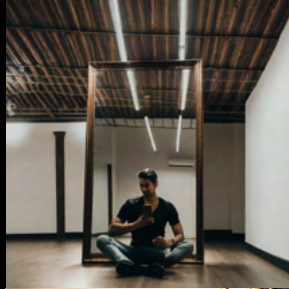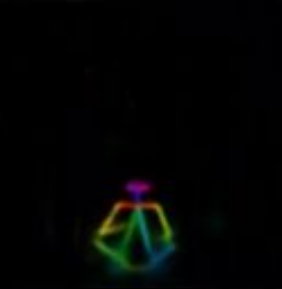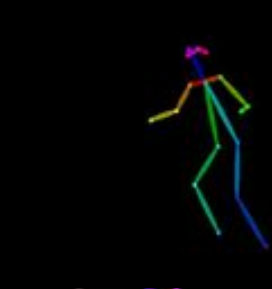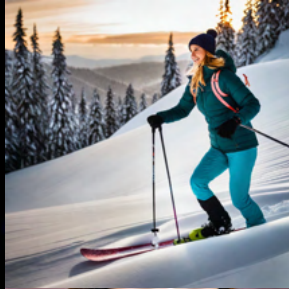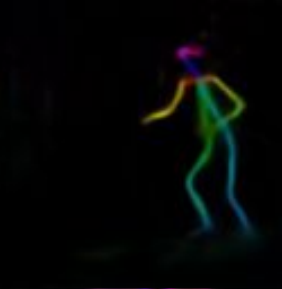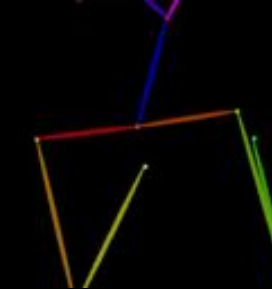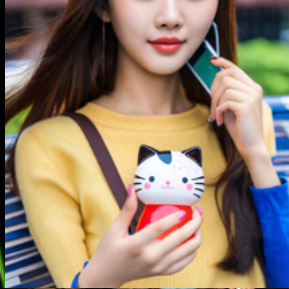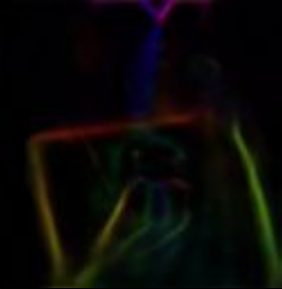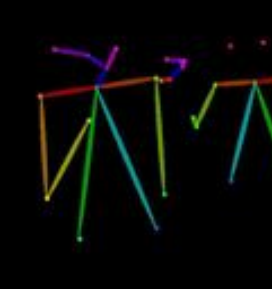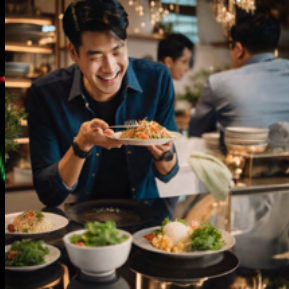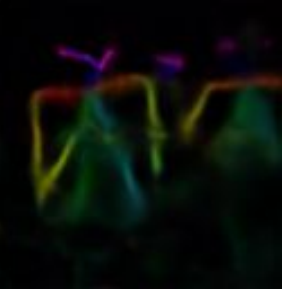



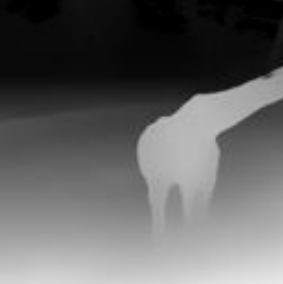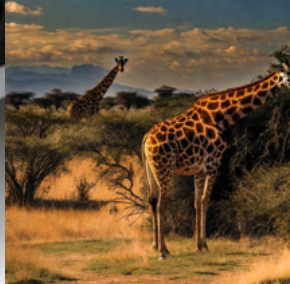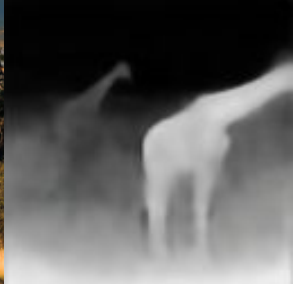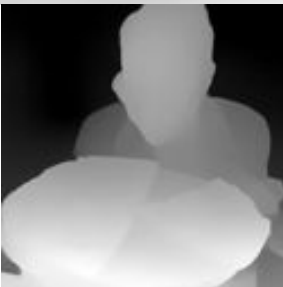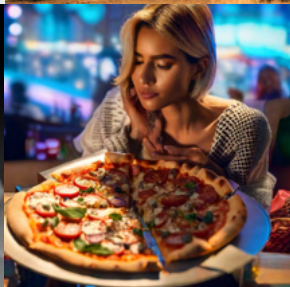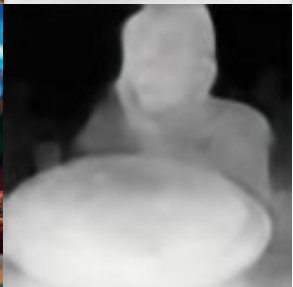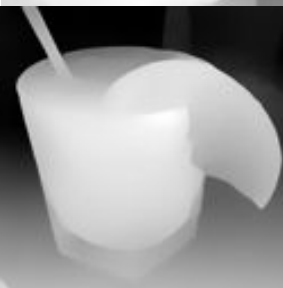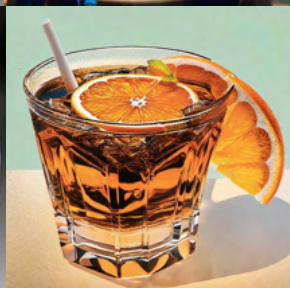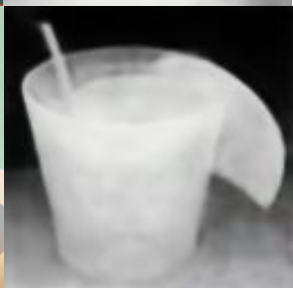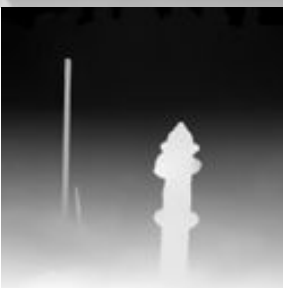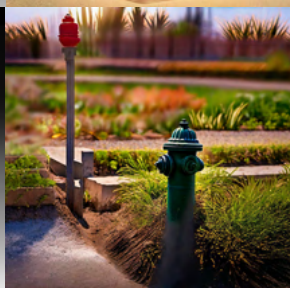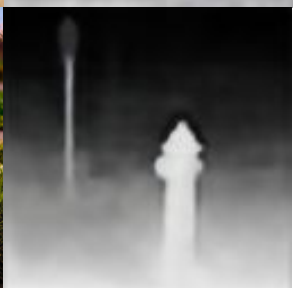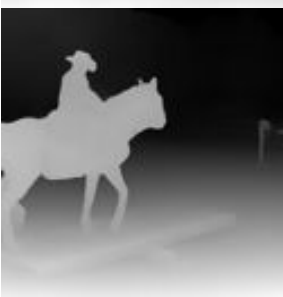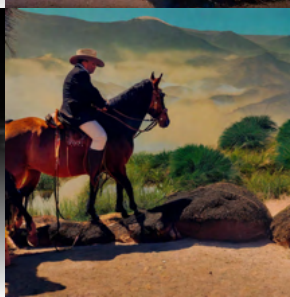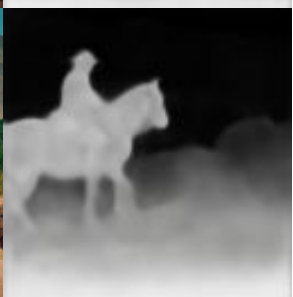

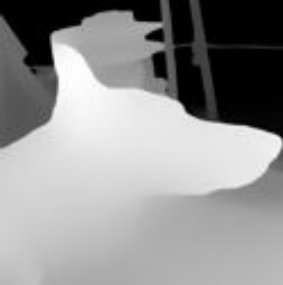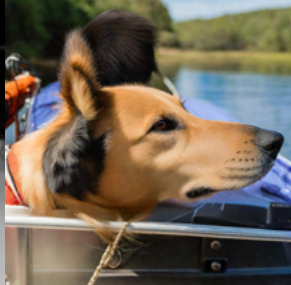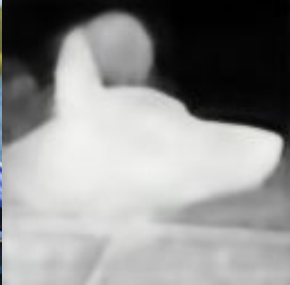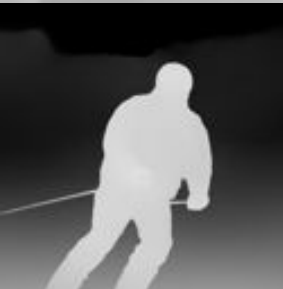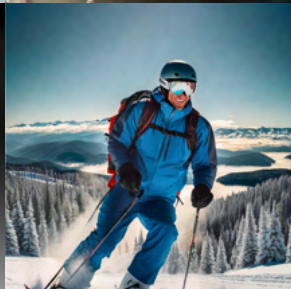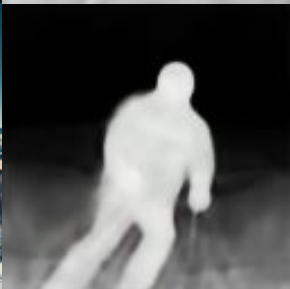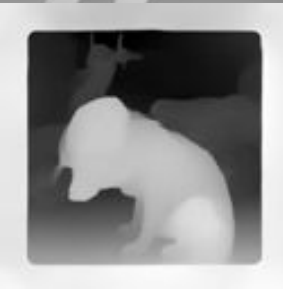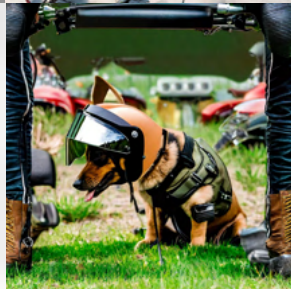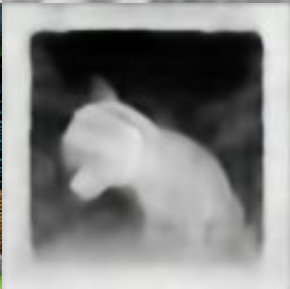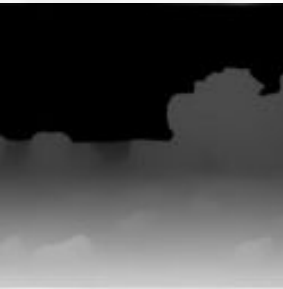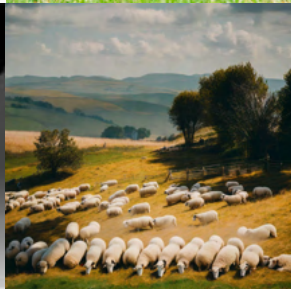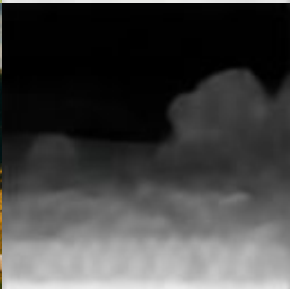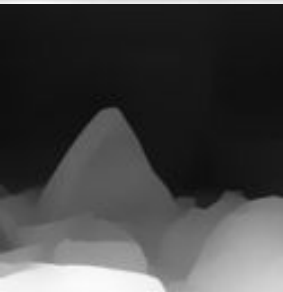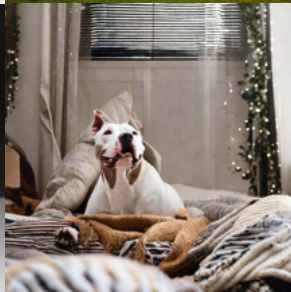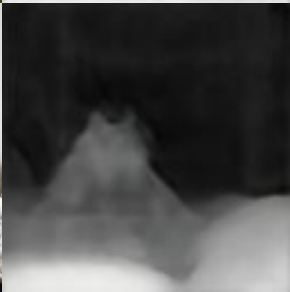

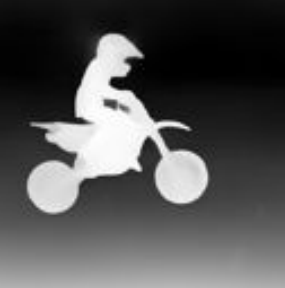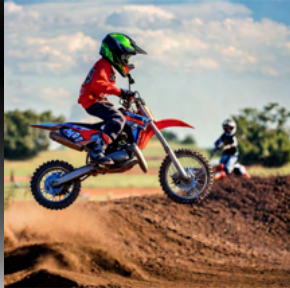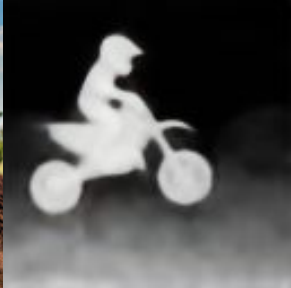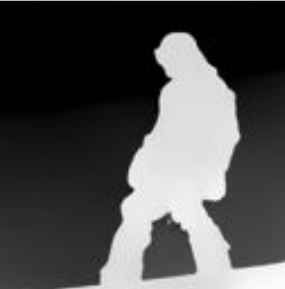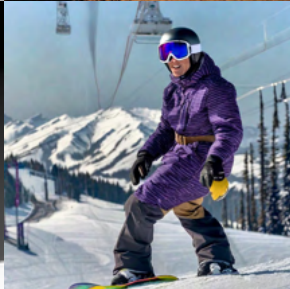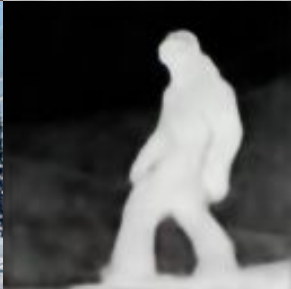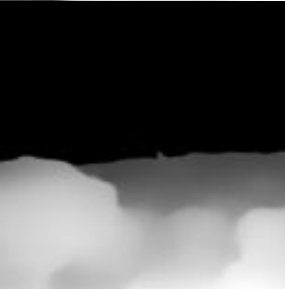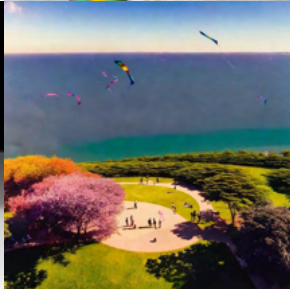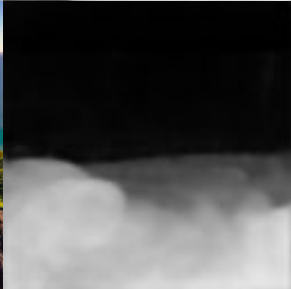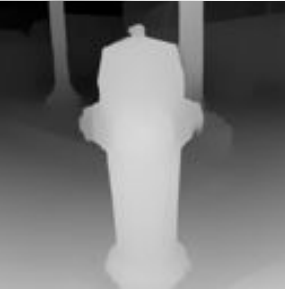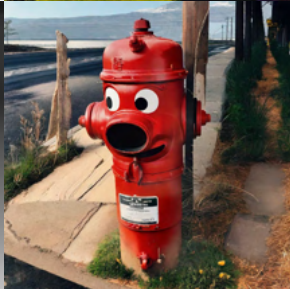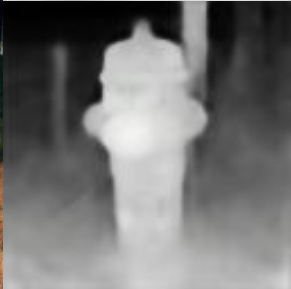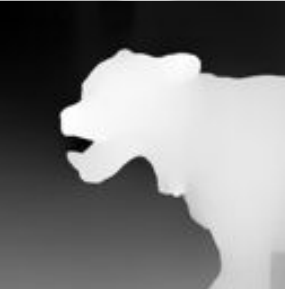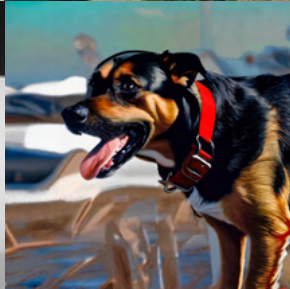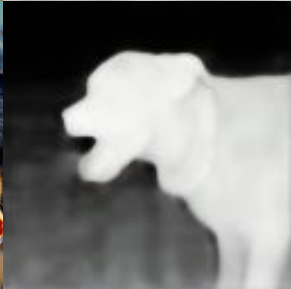

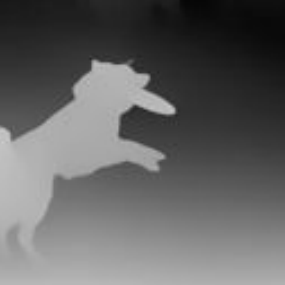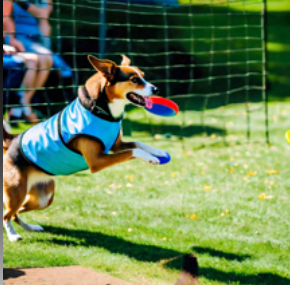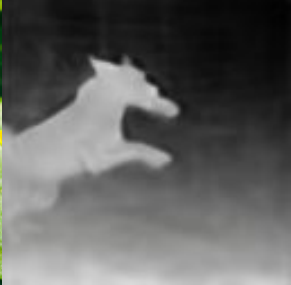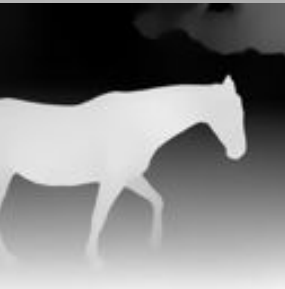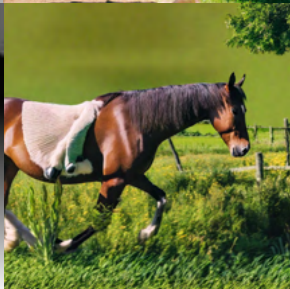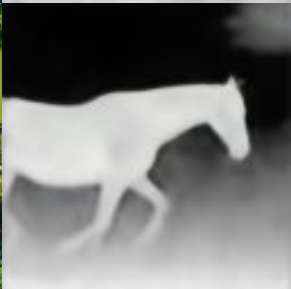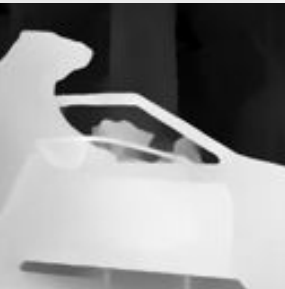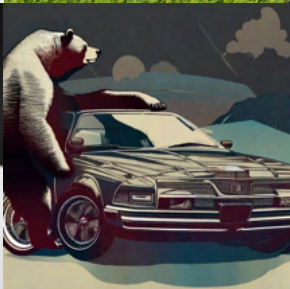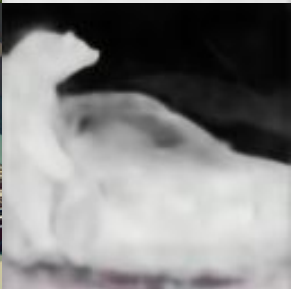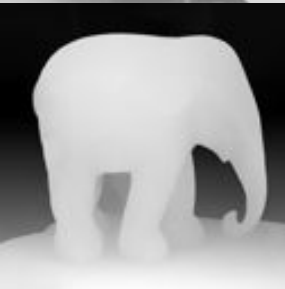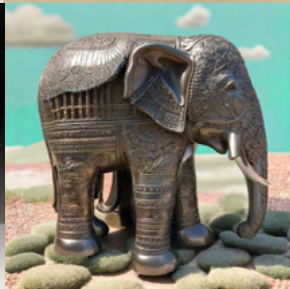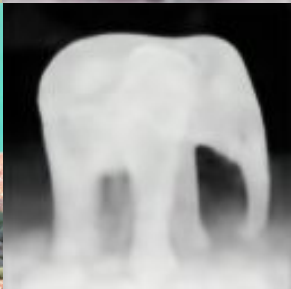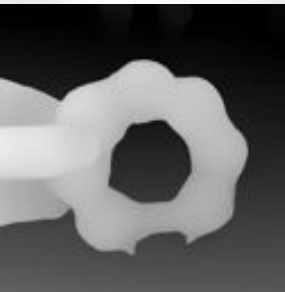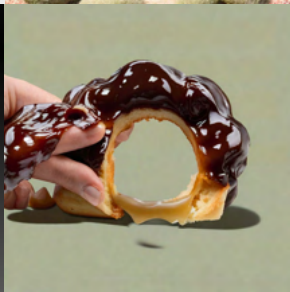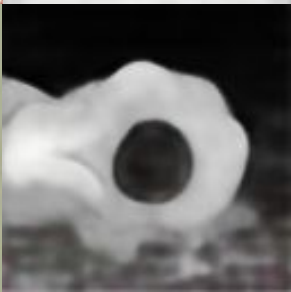



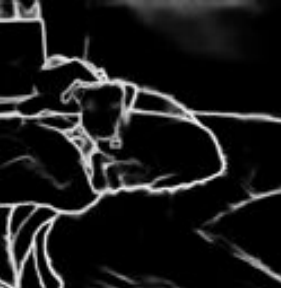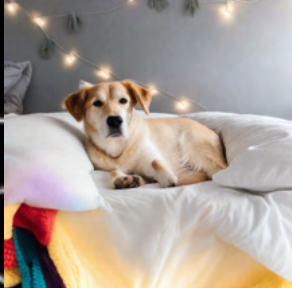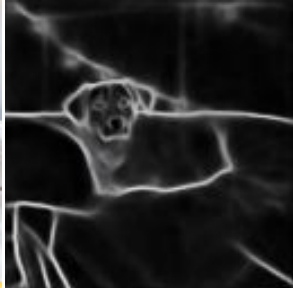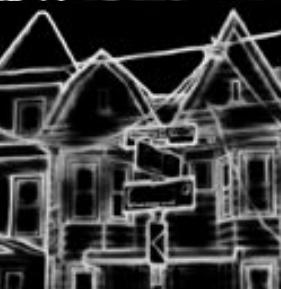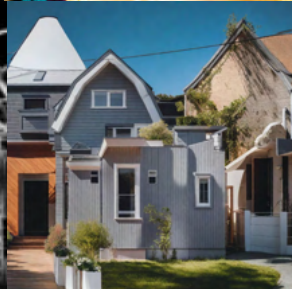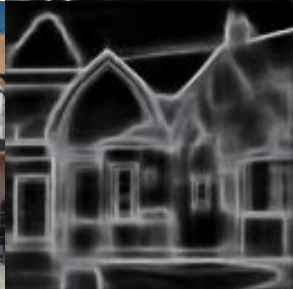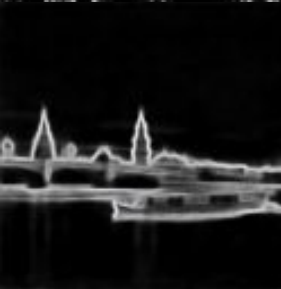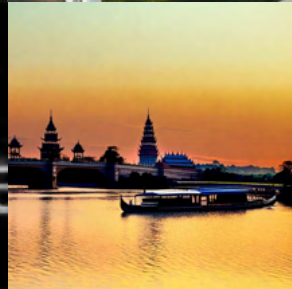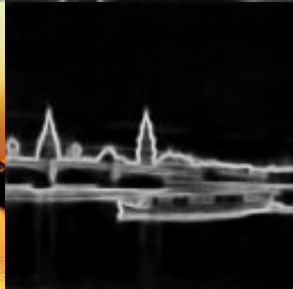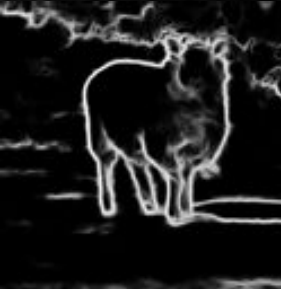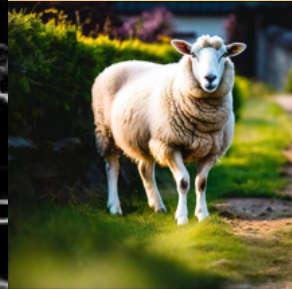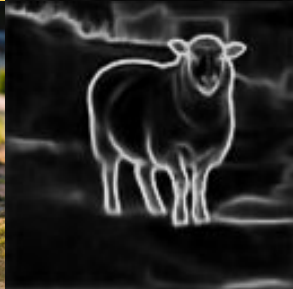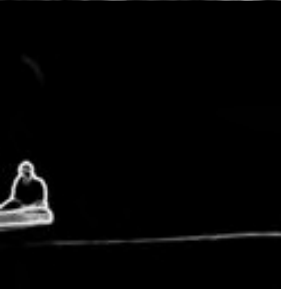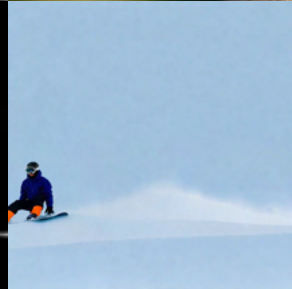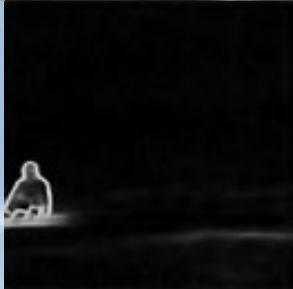

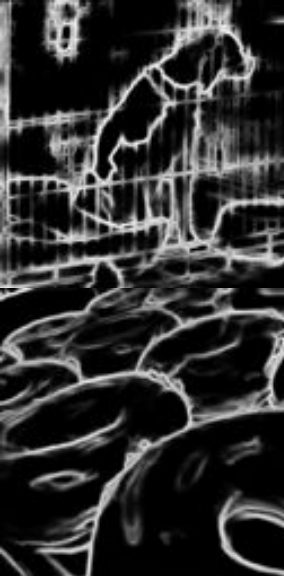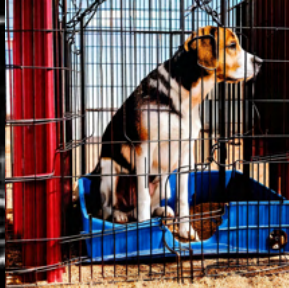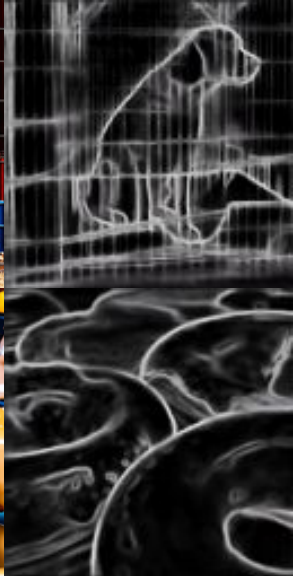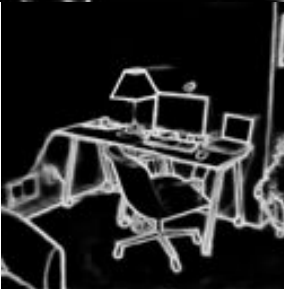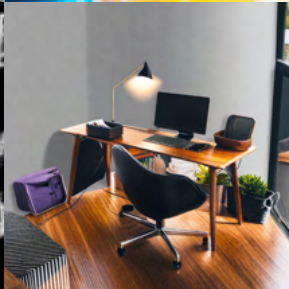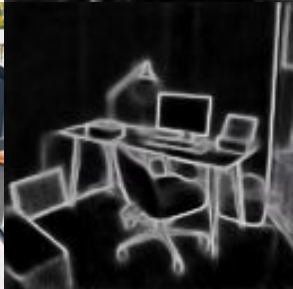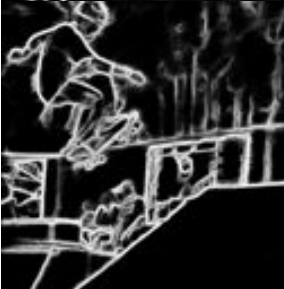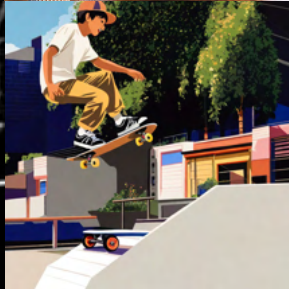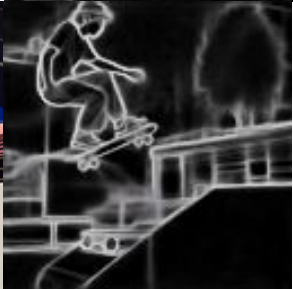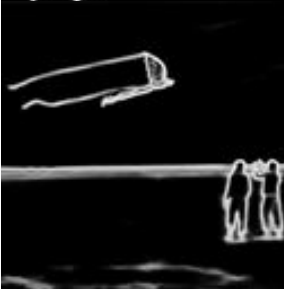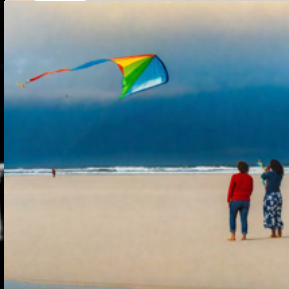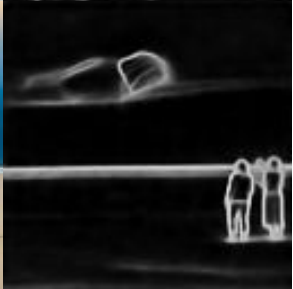

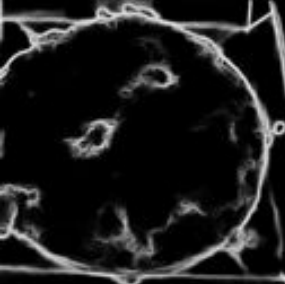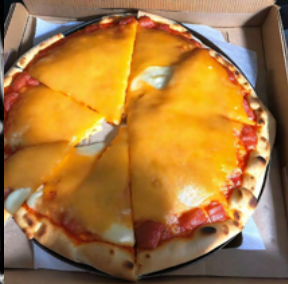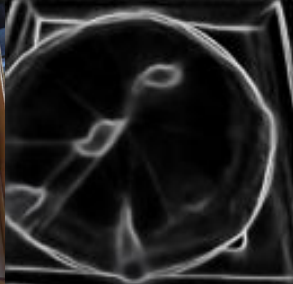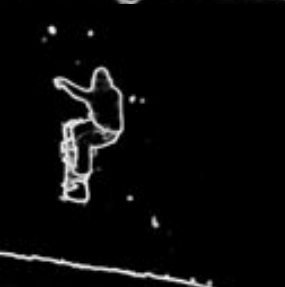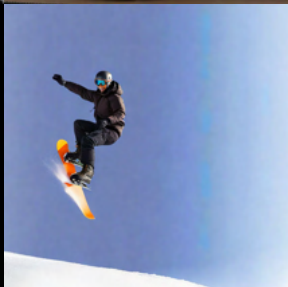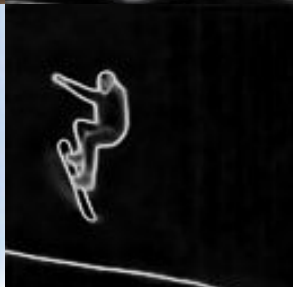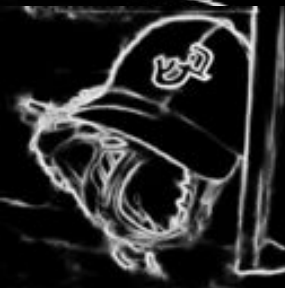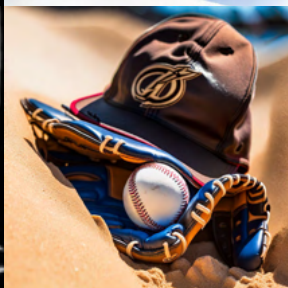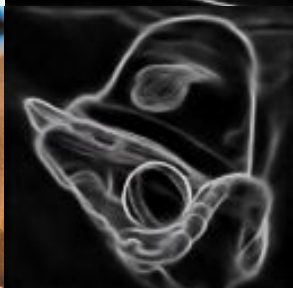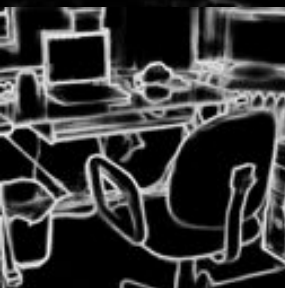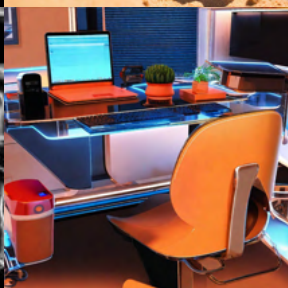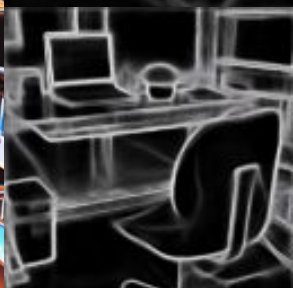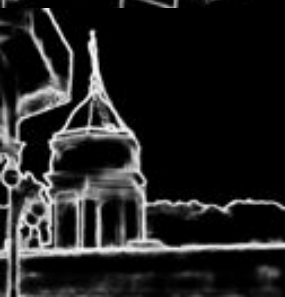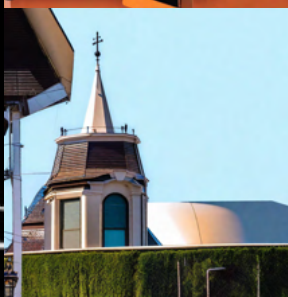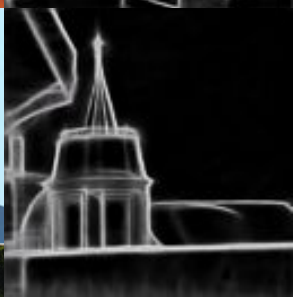



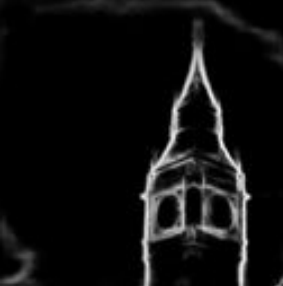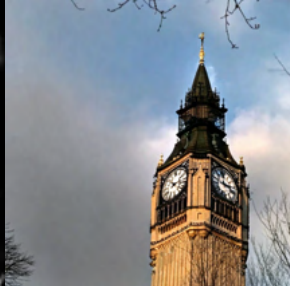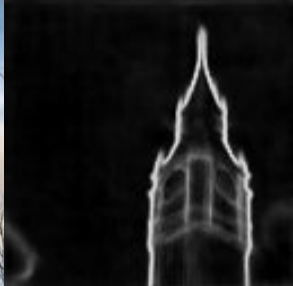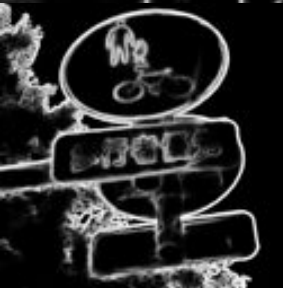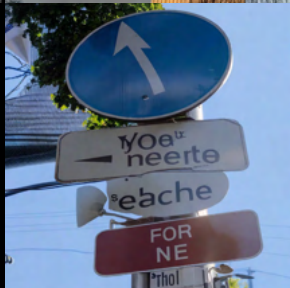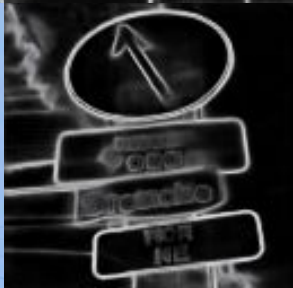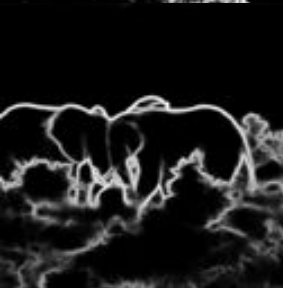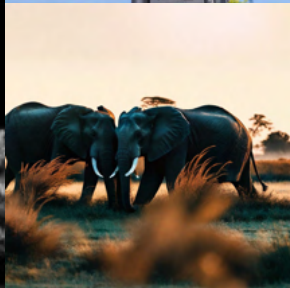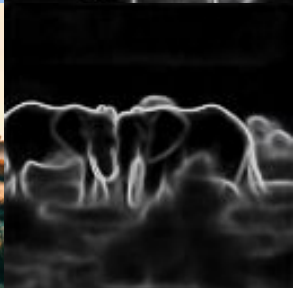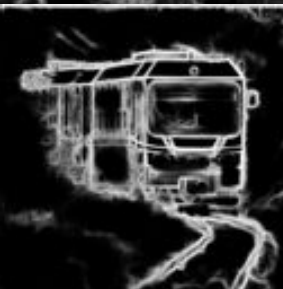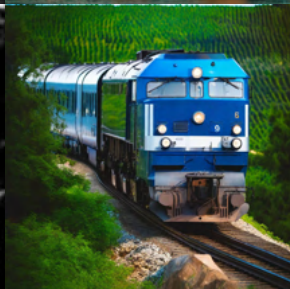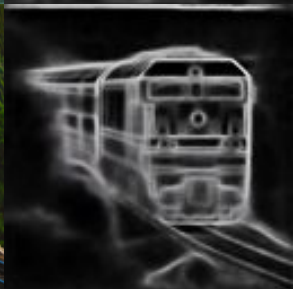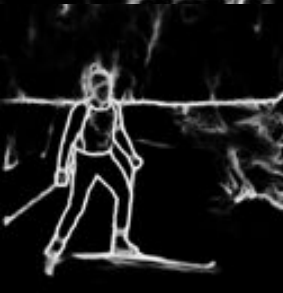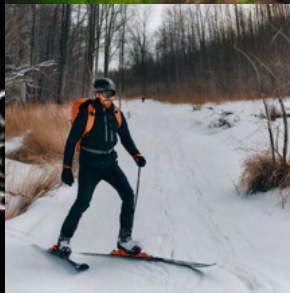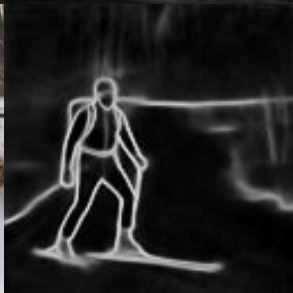

Supplement: Supplementary file 1 [file control_suppl.pdf]
