# Supplementary material for: Readout Guidance: Learning Control from Diffusion Features
Source: arXiv:2312.02150 source file (2024-04-02)

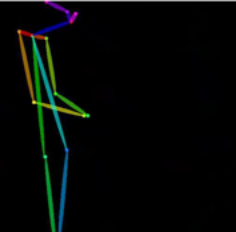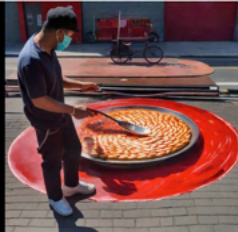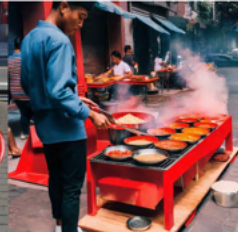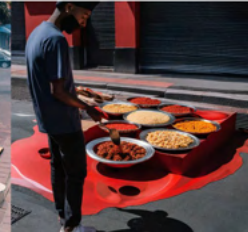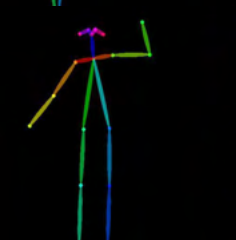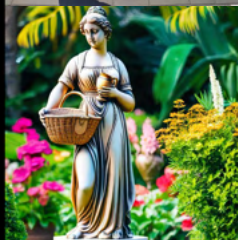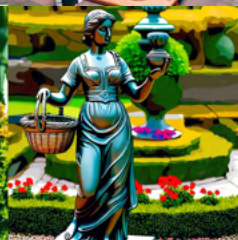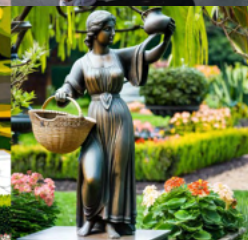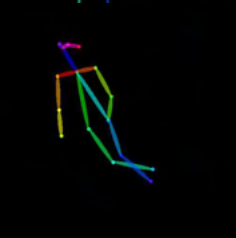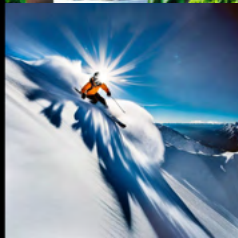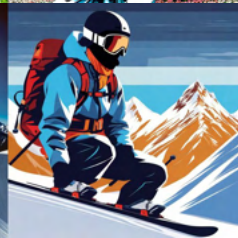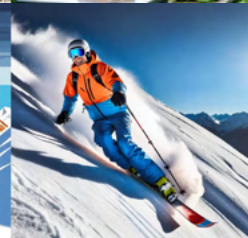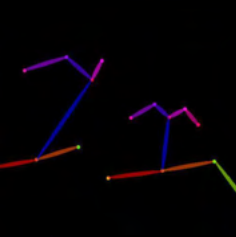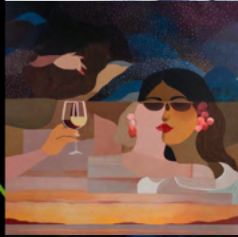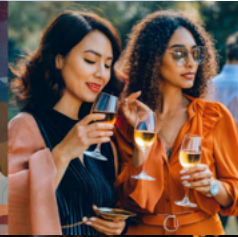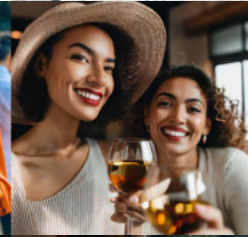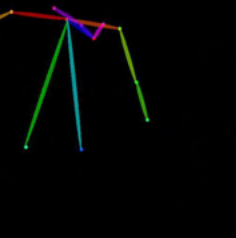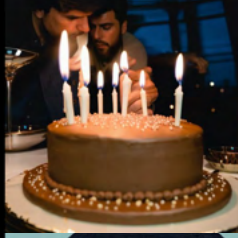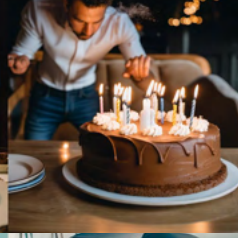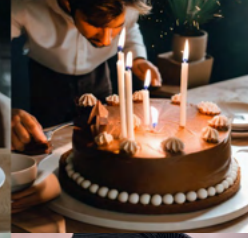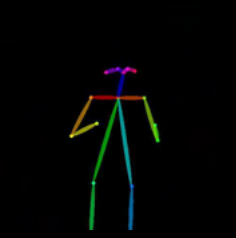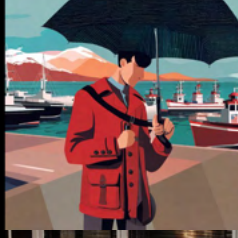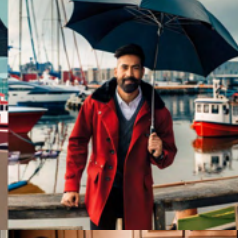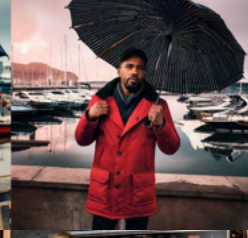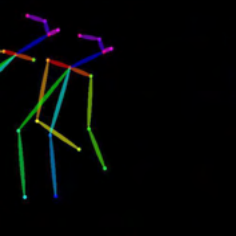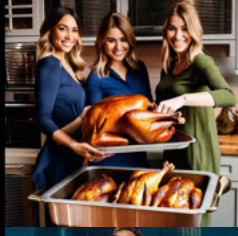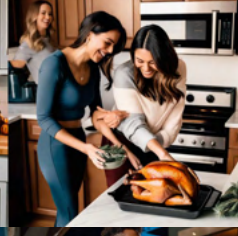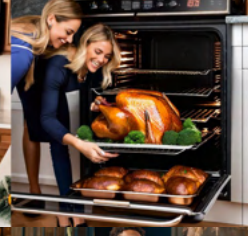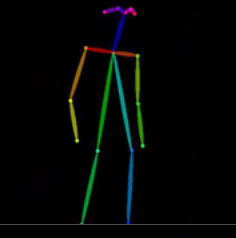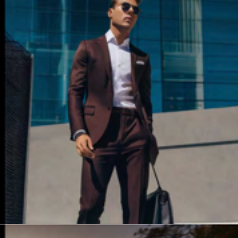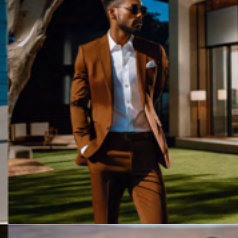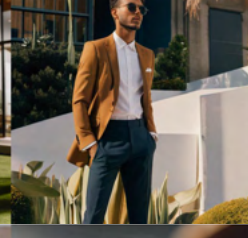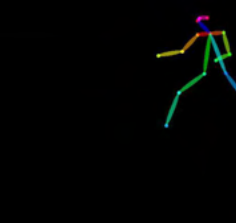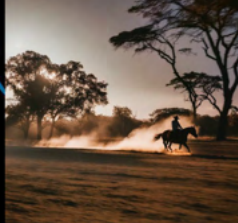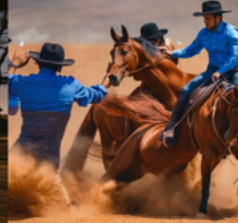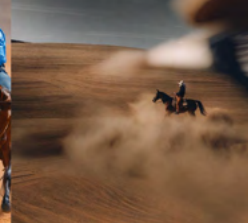



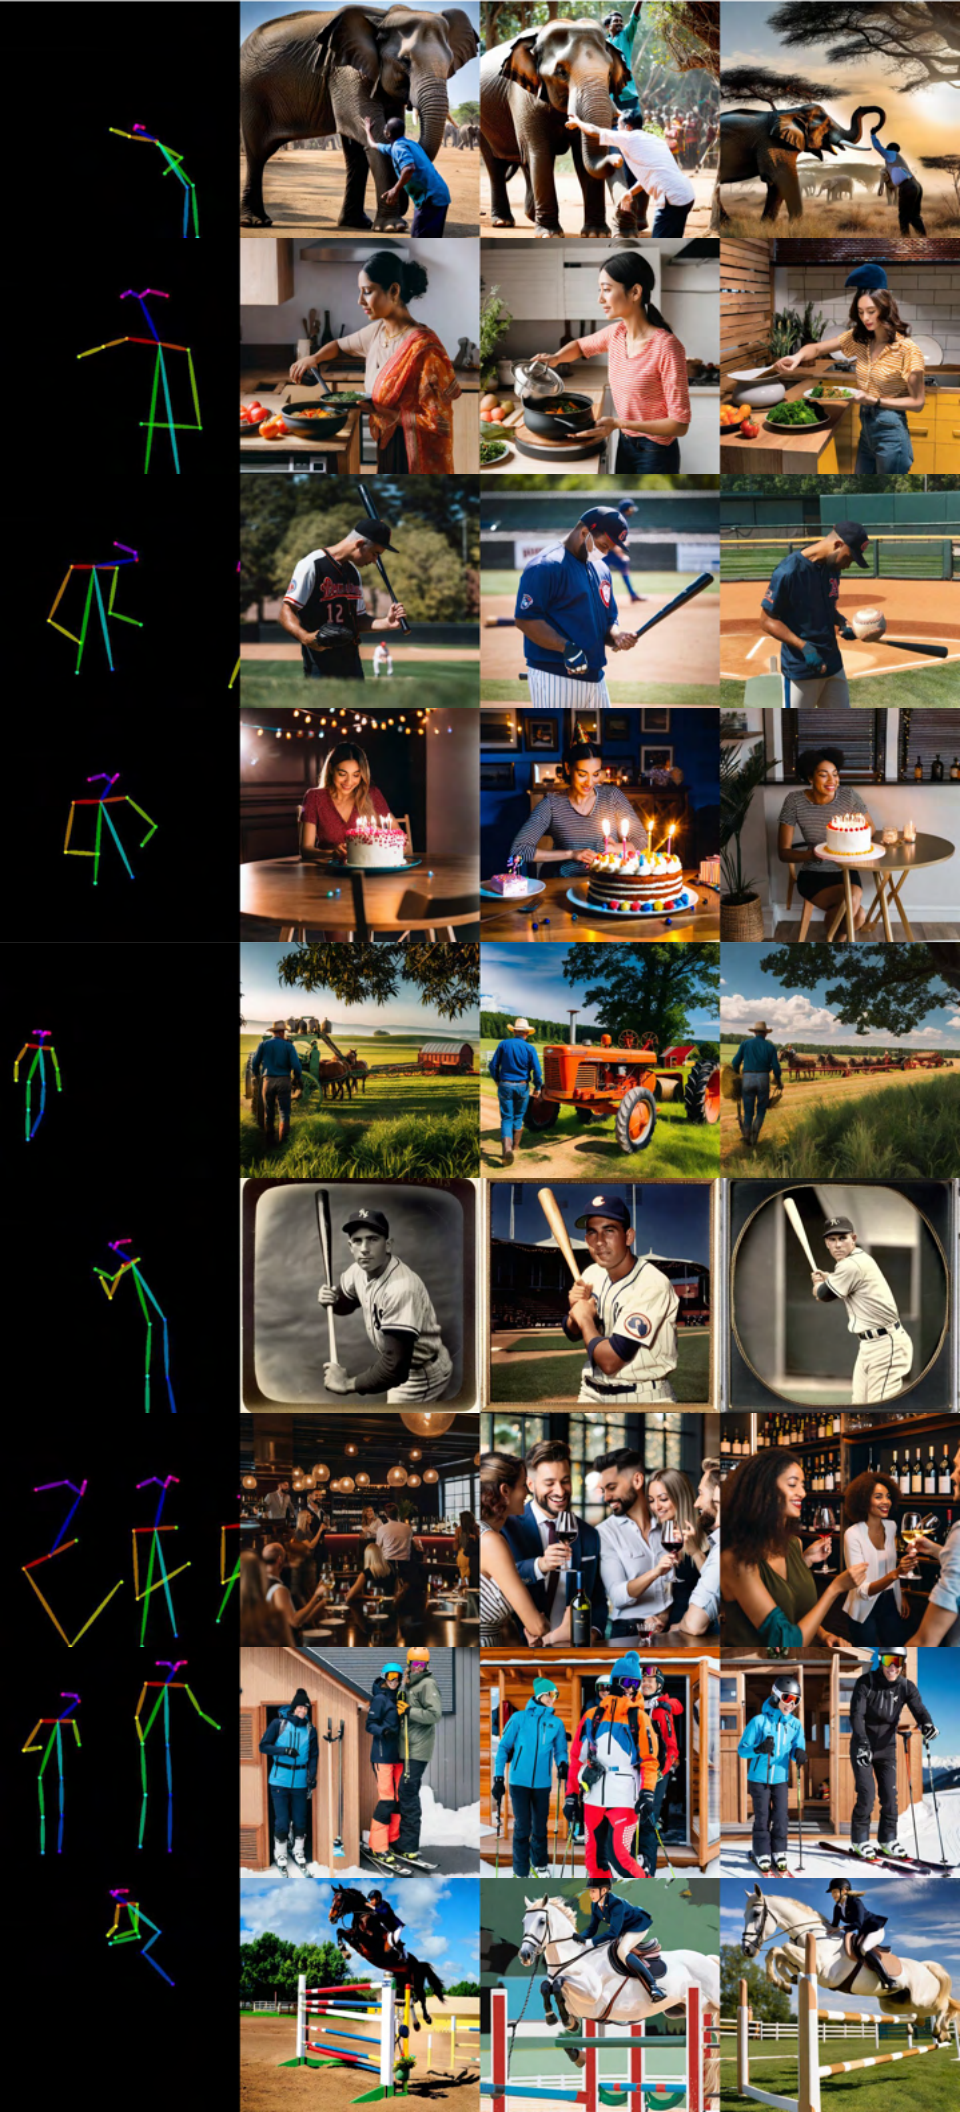

Supplement: Supplementary file 3 [file train_size_suppl.pdf]
